# Supplementary material for: Introducing Intermediate Domains for Effective Self-Training during Test-Time
Source: arXiv:2208.07736 source file (2022-11-08)
Supplement: Supplementary file 1 [file hyperparameters.tex]

\begin{table*}[h]

\centering
\caption{Hyperparameters used for CIFAR-C, ImageNet-C, ImageNet-R, and CarlaTTA. \textit{batch size (test)} denotes the number of unique test samples, whereas \textit{batch size (total)} consists of both source and test samples, used for one adaptation step.}
\label{tab:hyperparameters}
\begin{tabular}{lc|cccc}
    \hline
    && CIFAR-C & ImageNet-C & ImageNet-R & CarlaTTA \\
    \hline
    optimizer && Adam & Adam & Adam & SGD \\
    learning rate && 1e-5 & 1e-5 & 1e-5 & 2.5e-4\\
    momentum && - & - & - & 0.9 \\
    weight decay && - & - & - & 0.0005 \\
    batch size (test) && 200 & 64 & 64 & 1 \\
    weight & $\lambda_{\mathrm{ST}}$ & 1.0 & 1.0 & 1.0 & 0.1 \\
    \hline
\end{tabular}
\end{table*}
